# Supplementary material for: Inducing Predictive Uncertainty Estimation for Face Recognition
Source: arXiv:2009.00603 source file (2020-09-01)
Supplement: Supplementary file 1 [file appendix.tex]

%%%%%%%%%% Merge with supplemental materials %%%%%%%%%%
\clearpage
\setcounter{section}{0}
\vspace{10pt}
\begin{center}
\textbf{\Large Supplemental Materials}
\end{center}
%%%%%%%%%% Merge with supplemental materials %%%%%%%%%%
%%%%%%%%%% Prefix a "S" to all equations, figures, tables and reset the counter %%%%%%%%%%
\setcounter{equation}{0}
\setcounter{figure}{0}
\setcounter{table}{0}
\setcounter{page}{1}
\makeatletter

%%%%%%%%%% Prefix a "S" to all equations, figures, tables and reset the counter %%%%%%%%%%

% ------------------------------------------
\section{Architecture for PCNet}
Here, we present the backbone architecture for the proposed PCNet,
which is based on the standard ResNet18 with an extra fully connected layer at the end.
\input{./tables/architecture.tex}
% ------------------------------------------

% ------------------------------------------
\section{Generating pairwise verification scores}
As explained in Section.~\ref{sec:gen},
we first train a standard ResNet34 for face recognition on half of the VGGFace2 training set.
Once trained, verification scores are obtained for all mated pairs in the the other half of the dataset.
Some example verification scores are shown in Figure~\ref{fig:generate_pc}.
Two phenomenon can be observed,
\emph{First}, 
the images in the VGGFace2 dataset are of very diverse poses, resolutions and age ranges, 
making it perfect to train quality estimation models, 
\ie~there exists a large number of relatively low quality images, 
which potentially challenges the existing mid range face recognition systems.
\emph{Second}, 
the verifciation scores are only given both images in the pair are of high visual quality,
\eg~high resolution, frontal face.

% ------------------------------------------
\input{./figures/pipeline.tex}
% ------------------------------------------

\section{Visualization on single-image confidence scores}
\input{./figures/visualization_appendix.tex}

% ------------------------------------------
